# Supplementary material for: Scope of Pre-trained Language Models for Detecting Conflicting Health Information
Source: arXiv:2209.11102 source file (2022-09-22)
Supplement: Supplementary file 1 [file Supplementary.tex]

\section{Supplementary Materials}
\subsection{Medical Advice Dataset}
We use the annotated medical advice dataset shared and reported by the authors in \cite{PREUM2017226} to evaluate our solution. This dataset contains textual medical advice curated from authentic health websites, and mobile apps. It contains medical advice on a wide range of topics including general health topics (e.g., weight loss, pregnancy, exercise), and prevalent chronic diseases (e.g., chronic kidney disease, dementia, type 2 diabetes, hypertension, obesity). For collecting medical advice on a chronic disease, the authors considered both advice related to managing the disease and  advice related to the prescription medications used to treat the disease. The context of the data collection was increasing personalized health safety in terms of disease management and medications. 

For each advice, the dataset contains annotation of advice topics/objects, and  polarity of an advice with respect to a topic. It also contains pair of advice statements with conflict labels, i.e., type of conflict or no conflict. The pairs are constructed so that they have at least one common topic/object. The taxonomy of conflict type was constructed by consulting with multiple doctors employed in a local hospital. The dataset was annotated by three human annotators and the annotation was reviewed by multiple doctors. The overall inter-annotator agreement is 0.977 in terms of $\kappa$ score \footnote{$\kappa$ is scored between 0-1 and a higher value of $\kappa$ indicates higher agreement}. Additional details of the dataset can be found in \cite{PREUM2017226}.

% \subsection{Data Collection}
% how did we decide the high level topics?
%     general health topics --> mobile app --> #of topics, # of advice
%     chronic diseases prescription --> #of diseases, # of drugs, # of advice
%     how did we decide the sources of information:
% % need a flow chart?

% context of data collection: personalized health safety, patient age, medical history, mobile health. Noe solely ML / NLP

% \subsection{Data Annotation}
%     single advice: topics/ objects, sentiment, tokens, 
%     pair wise advice: conflict
%         how did we make the pairs?
%         # of potential pairs
%         how did we decide on the types of conflict
%             doctor's feedback
%         inter annotator agreement

\subsection{Effect of Data Augmentation}
\definecolor{maroon}{cmyk}{0,0.87,0.68,0.32}
\begin{table*}[!h]

\begin{tabularx}{\linewidth}{c c X X X}

\toprule
\# &\textbf{Augmentation} &\textbf{Advice 1}  & \textbf{Advice 2}\\ 
\midrule
1&None & Reduce the consumption of carbohydrates. & Increase your protein intake and also have more of carbohydrate in your diet.  \\
1&Pegasus & The consumption of sugars should be reduced. & You should have more of the two in your diet.  \\
1& Back Translate & Reduce the consumption of carbohydrates. & Increase your protein intake and also include more carbohydrates in your diet. \\
\rowcolor{maroon!10} 2&None & Combine exercise and diet. & Ditch the diet. \\
\rowcolor{maroon!10}2& Pegasus & You can combine exercise and diet.  & Don't eat the diet. \\
\rowcolor{maroon!10}2& Back Translate & Combine exercise and diet. & The diet is burying itself. \\
\bottomrule

\end{tabularx}
\caption{Failed augmentation examples for two different direct conflict samples. Rows 1 and 4 contain the original advice pairs with no augmentation. For each sample, we display how Pegasus and Back Translation augment the original samples. } 
\label{augmentation}
\end{table*}

% --cite other techniques
In effort to synthetically increase the size of our dataset, we experimented with various data augmentation strategies including abstractive summarization, contextual word embedding, natural language generation, and back-translation.
Of these approaches, we found the two which produced the most coherent outputs were abstractive summarization with Pegasus \cite{zhang2020pegasus}, and back-translation \cite{Sennrich2016ImprovingNM}. The goal when using Pegasus is to paraphrase an advice pair while preserving label correctness. Unfortunately, Pegasus fails when either (i) the conflict topic is altered (ii) the conflict topic is deleted (iii) the paraphrase is of poor quality. In sample 1 of Table \ref{augmentation} notice how for Advice 1, Pegasus does a good job at paraphrasing in terms of semantics and coherency, but changes the conflict topic (carbohydrates) to sugars. While the topic replacement is semantically similar, the label is no longer correct as Advice 2 may be referring to whole-grain carbohydrates such as rice or wheat, not necessarily sugary foods. In general, swapping out the conflict topic is dangerous given that all medical advice  in the MCD dataset are factual in their given context. Any altering of the advice topic thus requires explicit validation, which makes use of automatic augmentation strategies challenging. 
% mention why this would be a problem to preserve factual advice
In Advice 2, we see that Pegasus fails to capture the semantics of the original advice. Pegasus, however, does do a great job with Advice 2 of sample 2. Unfortunately, it is challenging to automatically detect what a good augmented sample is, making it tough to identify good paraphrasings when so many have significant issues. 

For back translation, we often struggle with generating samples that provide textual diversity as shown in Table \ref{augmentation}. In sample 1, Advice 1 back translated outputs the same text while Advice 2 only changes a few semantically irrelevant terms. In sample 2, we similarly find the back translation produces no change, while Advice 2 back translated produces a nonsensical output. 

The issues described above occur frequently in our augmentation experiments, making it challenging to generate augmented samples for our dataset. 

\subsection{Hardware Specifications}
All experiments in this study were run on Google Colab. Our models were trained on a Tesla P100 GPU, Intel(R) Xeon(R) CPU @ 2.30GHz with 16GB RAM. 

\subsection{Hyperparameters}
In general, we did not perform hyperparameter optimization on any models presented in this study. Rather, we used the default training hyperparameters provided by Huggingface \cite{wolf-etal-2020-transformers}. 
One exception is that each model was trained for a maximum of 10 epochs with an early stopping patience of 3. Fine-tuning for only 3 epochs, which is the Huggingface default value, we found may not give our model enough time to learn representations for the relations matrix $E$, for which we build relational representations from scratch.  

Given the sensitivity of our models to weight initialization, performing any sort of thorough parameter search would have taken considerable resources as, if we need to run $n$ trials to perform a single experiment (which reports a mean statistic) and $m$ experiments to search for a single hyperparameter, hyperparameter search soon becomes a very expensive task. Thus, proper hyperparameter search is out-of-scope of this paper and will be explored in the future.

\begin{figure}[!h]
    \centering
    \includegraphics{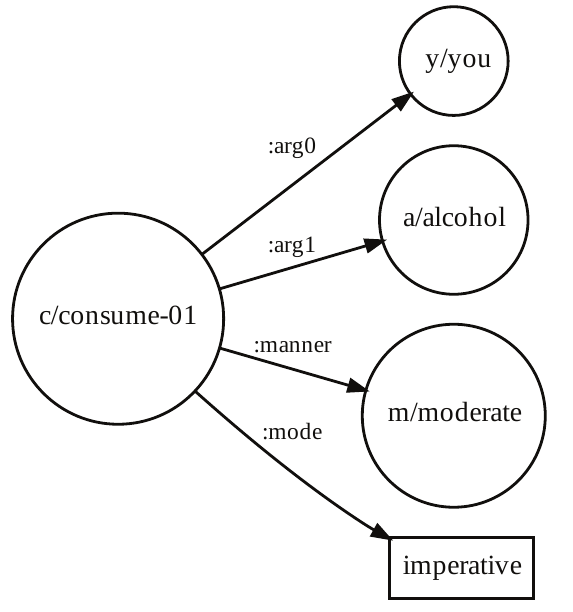}
    \caption{Example AMR graph for the advice ``Consume alcohol in moderation." This graph was generated using a SOTA AMR parser. }
    \label{amr_example}
\end{figure}

\subsection{Relations Matrix}
\ModelName uses a relations matrix $E$ to relate two tokens $W_i, W_j$ to one another using an AMR graph. Most details on how this matrix is constructed can be found in \cite{AMR_Dialogue}, however there are some adjustments we make for our input structure. Below, we provide a high-level outline of how $E$ is constructed: \\

\noindent For a given $W_i, W_j$ in our tokenized input:
\begin{enumerate}
    \item If $i \neq j$ and $W_i$ is related to $W_j$ in the AMR graph, with some relation $r$, then $E_{ij} = r$. If $r$ is not in the training set's AMR vocabulary, then $E_{ij} = \mathrm{<unk>}$. 
    \item If $i = j$, $E_{ij} = \mathrm{self}$ as described in \cite{AMR_Dialogue}. However, if $W_i$ modifies $W_j$, we use the modifying relation instead of `self'. For example, in Figure \ref{amr_example}, \textit{imperative} is a modifier of \textit{consume}, not a separate AMR concept. Since this information is not captured naturally in $E$, we replace `self' with the modifier when one is available. 
    \item Each token is informed of where the beginning of each sentence is with a `bos' relation. Practically, this points to the [CLS] token for Advice 1, and the first [SEP] token for Advice 2. 
    \item If $i \neq j$ and $W_i$ is not related to $W_j$, then $E_{ij} = \mathrm{None}$. 
    \item The BERT tokenizer will break down words into sub-tokens if the full word is not in it's full vocabulary. Thus, if a word is broken down and has an AMR relation, we duplicate this relation for all sub-tokens. For example, consider two words $W^i = \{W^i_0, \dots ,W^i_n\}$ and  $W^j = \{W^j_0 \dots ,W^j_m\}$, where the corresponding sets for each word represent the BERT tokenized version of the word. In our formulation, if $W^i$ is related to $W^j$ through some relation $r$ via the AMR graph, then $$E_{i+a, j+b} = r \:\: \mathrm{for \: all\: } {W_a} \in W^i, {W_b}\in W^j$$
  
    \end{enumerate}
