# Supplementary material for: Scope of Pre-trained Language Models for Detecting Conflicting Health Information
Source: arXiv:2209.11102 source file (2022-09-22)
Supplement: Supplementary file 2 [file 9Appendix.tex]

\section{Appendix}
\subsection{Additional Dataset Details}
In Figure \ref{fig:data_flow}, we highlight details of the data collection process. Specifically, to expand the PreCluDe dataset, we first scraped various online health platforms for potential health advice statements. Of the 47,600 collected health texts, we had researchers at the submitting author's institution annotate 5393 of the texts as ``Useful" or ``Not Useful". Useful texts were legitimate advice statements, while Not Useful texts were statements of fact or other information with no actionable health advice. 2715 of these texts were found to be Useful for HCD, and from this set we produced 1897 advice pairs for our final dataset. 

The PreCluDe dataset contains 3285 unique advice statements, from which we utilize 2006 HCD samples. Note that more advice pairs are available in PreCluDe for rare conflict types such as quantitative conflicts. However, these were excluded from our dataset and maybe explored in future works.  
\begin{figure}[!h]
    \centering
    \includegraphics[scale = 0.23]{Figures/Dataflow Diagram v2.png}
    \caption{Data flow diagram for HCD data collection and dataset formation. }
    \label{fig:data_flow}
\end{figure}
